# Supplementary material for: CLEVRER: CoLlision Events for Video REpresentation and Reasoning
Source: arXiv:1910.01442 source file (2020-03-08)
Supplement: Supplementary file 1 [file supp.pdf]

# Supplementary Material

## A. Descriptive Question Sub-types and Statistics

Descriptive questions in CLEVRER consists of five sub-types. When generating the questions, we balance the frequency of the answers within each question sub-type to reduce bias. The sub-types and their answer space distribution are summarized in Figure 1.

| Sub-type       | Answers                                             |
|----------------|-----------------------------------------------------|
| Count          | 0, 1, 2, 3, 4, 5                                    |
| Exist          | yes, no                                             |
| Query_material | rubber, metal                                       |
| Query_shape    | sphere, cube, cylinder                              |
| Query_color    | gray, brown, green, red, blue, purple, yellow, cyan |

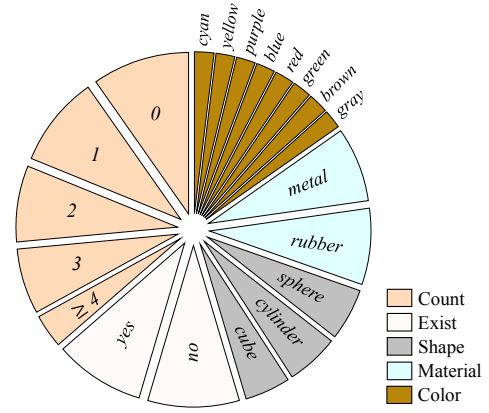

Figure 1: Descriptive question sub-type and answer space statistics.

## B. Model Details

**Question parser.** The program parser of the DEPICTR model consists of an LSTM encoder and an LSTM decoder. Given an input word sequence  $(x_1, x_2, \dots, x_I)$ , the encoder first generate a bi-directional latent encoding at each step:

$$e_i^f, h_i^f = \text{LSTM}(\Phi_I(x_i), h_{i-1}^f), \quad (1)$$

$$e_i^b, h_i^b = \text{LSTM}(\Phi_I(x_i), h_{i+1}^b), \quad (2)$$

$$e_i = [e_i^f, e_i^b]. \quad (3)$$

The decoder then generates a sequence of program tokens  $(y_1, y_2, \dots, y_J)$  from the latent encodings using attention:

$$v_j = \text{LSTM}(\Phi_O(y_{j-1})), \quad (4)$$

$$\alpha_{ji} \propto \exp(v_j^T e_i), \quad c_j = \sum_i \alpha_{ji} e_i, \quad (5)$$

$$\hat{y}_j \sim \text{softmax}(W \cdot [q_j, c_j]). \quad (6)$$

At training time, the input program tokens  $\{y_j\}$  are used for generating the predicted labels  $y_{j-1} \rightarrow \hat{y}_j$  at each step  $j = 1, 2, 3, \dots, J$ . The generated label  $\hat{y}_j$  is then compared with  $y_j$  to compute a loss for training. At test time, the decoder rolls out by feeding the sampled prediction at the previous step to the input of the current step  $\hat{y}_j = y_j$ . The roll-out stops when the end token appears or when the sequence reaches certain maximal length.

**Dynamics predictor.** We use the Propagation Network (PropNet) [2] for predicting motion and event traces. The notation, dynamics representation and basic modules are defined in Section 4 in the main text. Here we show how PropNet makes predictions over the dynamics by propagating the influences through the interaction graph.

At time  $t$ , we first encodes the objects  $c_{i,t}^o = f_O^{\text{enc}}(o_{i,t})$ , and relations  $c_{k,t}^r = f_R^{\text{enc}}(o_{u_k,t}, o_{v_k,t}, a_k^r)$ , where  $o_{i,t}$  denotes the information of object  $i$  at time  $t$ . We then denotes the propagating influence from relation  $k$  at propagation step  $l$  as  $e_{k,t}^l$ , and

the influence from object  $i$  as  $h_{i,t}^l$ . For step  $1 \leq l \leq L$ , propagations can be described as

Step 0:

$$h_{i,t}^0 = \mathbf{0}, \quad i = 1 \dots |O|, \quad (7)$$

Step  $l = 1, \dots, L$ :

$$\begin{aligned} e_{k,t}^l &= f_R(c_{k,t}^r, h_{u_k,t}^{l-1}, h_{v_k,t}^{l-1}), \quad k = 1 \dots |R|, \\ h_{i,t}^l &= f_O(c_{i,t}^o, \sum_{k \in \mathcal{N}_i} e_{k,t}^{l-1}, h_{i,t}^{l-1}), \quad i = 1 \dots |O|, \end{aligned} \quad (8)$$

Output:

$$\begin{aligned} \hat{r}_{k,t+1} &= f_R^{\text{pred}}(c_{k,t}^r, e_{k,t}^L), \quad k = 1 \dots |R|, \\ \hat{o}_{i,t+1} &= f_O^{\text{pred}}(c_{i,t}^o, h_{i,t}^L), \quad i = 1 \dots |O| \end{aligned} \quad (9)$$

where  $f_O$  denotes the object propagator,  $f_R$  denotes the relation propagator, which are shared among the propagation steps.  $\mathcal{N}_i$  denotes the relations where object  $i$  is the receiver. We train the neural dynamics predictor by minimizing the  $\mathcal{L}_2$  distance between the predicted  $\hat{r}_{k,t+1}, \hat{o}_{i,t+1}$  and the real future observation  $r_{k,t+1}, o_{i,t+1}$  using stochastic gradient descent.

**Program executor.** The program executor includes a collection of functional modules implemented in Python. Given an input program, the modules form a tree-structured execution trace. Each leaf inputs either a set of objects or events. When passing through the tree branch, the modules along the path are executed sequentially, performing logic operations and filtering on the input set of objects/events and passing the output to the following modules. Some modules join tree branches by taking more than one inputs. At the root of the program is an output module that returns the answer to the question. For descriptive type questions, the programs are executed directly; for open-ended questions, the executor first executes the program of the target option, and then executes the program of the question to obtain a “yes”, “no” token that indicates whether or not to select the option. A comprehensive list of all modules in the DEPICTR program executor is summarized in Table 1, and their input/output data types are summarized in Table 2.

## C. Implementation and Training Details

**Video frame parser.** Our frame parser is trained on 4,000 frames randomly selected from the training videos plus ground-truth masks and attribute annotations of the objects. We train the model for 30,000 iterations with stochastic gradient decent, using a batch size of 6 and learning rate 0.001. We keep the object proposals with a confidence score of  $> 0.9$  and use those to form the object-level abstract representation of the video.

**Neural dynamics predictor.** Our neural dynamics predictor is trained on the *proposed* object masks and attributes from the frame parser. We filter out inconsistent object proposals by matching the object intrinsic attributes across different frames and keeping the ones that appear in more than 10 frames. We normalize the input data to the range of  $[-1, 1]$  and concatenate them over a time window of size 3. We set the propagation step  $L$  to 2, and the dimension of the propagating effects  $D_{\text{enc}}$  to 512. We use the Adam optimizer [1] with an initial learning rate of  $10^{-4}$ , and a decay factor of 0.3 per 3 epochs. The model is trained for 9 epochs with batch size 2.

**Question parser.** For open-ended descriptive questions, the question parser is trained on 500 randomly selected question-program pairs. For multiple choice questions, we separately train the question parser on 500 questions and the choice parser 2,000 choices. The models are trained using Adam for 20,000 iterations with batch size 64 and learning rate  $7 \times 10^{-4}$ .

## D. Extra examples from the dataset

We show extra samples of CLEVRER’s videos and questions and DEPICTR’s results in Figure 2 through Figure 5.

## References

- [1] D. P. Kingma and J. Ba. Adam: A method for stochastic optimization. In *ICLR*, 2015. 2
- [2] Y. Li, J. Wu, J.-Y. Zhu, J. B. Tenenbaum, A. Torralba, and R. Tedrake. Propagation networks for model-based control under partial observation. *arXiv:1809.11169*, 2018. 1

| Module Type           | Name              | Input Type                 | Output Type           | Description                                                                                                   |
|-----------------------|-------------------|----------------------------|-----------------------|---------------------------------------------------------------------------------------------------------------|
| Input Modules         | Objects           | -                          | <i>objects</i>        | Returns all objects in the video                                                                              |
|                       | Events            | -                          | <i>events</i>         | Returns all events that happen in the video                                                                   |
|                       | UnseenEvents      | -                          | <i>events</i>         | Returns all future events after the video ends                                                                |
|                       | AllEvents         | -                          | <i>events</i>         | Returns all possible events on / between any objects                                                          |
|                       | Start             | -                          | <i>event</i>          | Returns the special “start” event                                                                             |
|                       | End               | -                          | <i>event</i>          | Returns the special “end” event                                                                               |
| Object Filter Modules | Filter_color      | <i>(objects, color)</i>    | <i>objects</i>        | Selects objects from the input list with the input color                                                      |
|                       | Filter_material   | <i>(objects, material)</i> | <i>objects</i>        | Selects objects from the input list with the input material                                                   |
|                       | Filter_shape      | <i>(objects, shape)</i>    | <i>objects</i>        | Selects objects from the input list with the input shape                                                      |
|                       | Filter_move       | <i>(objects, frame)</i>    | <i>objects</i>        | Selects all moving objects in the input frame                                                                 |
|                       | Filter_stationary | <i>(objects, frame)</i>    | <i>objects</i>        | Selects all stationary objects in the given frame                                                             |
| Event Filter Modules  | Filter_in         | <i>(events, objects)</i>   | <i>events</i>         | Selects all incoming events of the input objects                                                              |
|                       | Filter_out        | <i>(events, objects)</i>   | <i>events</i>         | Selects all exiting events of the input objects                                                               |
|                       | Filter_collision  | <i>(events, objects)</i>   | <i>events</i>         | Selects all collisions that involve any of the input objects                                                  |
|                       | Filter_before     | <i>(events, event)</i>     | <i>events</i>         | Selects all events before the target event                                                                    |
|                       | Filter_after      | <i>(events, event)</i>     | <i>events</i>         | Selects all events after the target event                                                                     |
|                       | Filter_order      | <i>(events, order)</i>     | <i>event</i>          | Selects the event at the specific time order                                                                  |
|                       | Filter_ancestor   | <i>event</i>               | <i>events</i>         | Returns all ancestors of the input event in the causal graph                                                  |
|                       | Get_frame         | <i>event</i>               | <i>frame</i>          | Returns the frame of the input event in the video                                                             |
|                       | Get_counterfact   | <i>object</i>              | <i>events</i>         | Returns all events after removing the input object                                                            |
|                       | Get_col_partner   | <i>(event, object)</i>     | <i>object</i>         | Returns the collision partner of the input object (the input event must be a collision)                       |
|                       | Get_in_out_object | <i>event</i>               | <i>object</i>         | Returns the object that participates in the input event (the input event must be a incoming / outgoing event) |
|                       | Unique            | <i>events / objects</i>    | <i>event / object</i> | Returns the only event / object in the input list                                                             |
| Output Modules        | Query_color       | <i>object</i>              | <i>color</i>          | Returns the color of the input object                                                                         |
|                       | Query_material    | <i>object</i>              | <i>material</i>       | Returns the material of the input object                                                                      |
|                       | Query_shape       | <i>object</i>              | <i>shape</i>          | Returns the shape of the input object                                                                         |
|                       | Count             | <i>objects</i>             | <i>int</i>            | Returns the number of the input objects                                                                       |
|                       | Exist             | <i>objects</i>             | <i>bool</i>           | Returns “yes” if the input objects is not empty                                                               |
|                       | Not               | <i>bool</i>                | <i>bool</i>           | Returns the opposite of the input boolean token                                                               |

Table 1: Functional modules of DEPICTR’s program executor. The `UnseenEvents` module takes predictive roll-outs from the dynamics predictor as input. The `Get_counterfact` module takes counterfactual roll-outs as input.

| Data type       | Description                                                                                            |
|-----------------|--------------------------------------------------------------------------------------------------------|
| <i>object</i>   | A dictionary storing the intrinsic attributes of an object in a video                                  |
| <i>objects</i>  | A list of <i>objects</i>                                                                               |
| <i>event</i>    | A dictionary storing the type, frame, and participating objects of an event                            |
| <i>events</i>   | A list of <i>events</i>                                                                                |
| <i>color</i>    | A string indicating a color out of “gray”, “brown”, “green”, “red”, “blue”, “purple”, “yellow”, “cyan” |
| <i>material</i> | A string indicating a material out of “metal”, “rubber”                                                |
| <i>shape</i>    | A string indicating a shape out of “cube”, “cylinder”, “sphere”                                        |
| <i>frame</i>    | An integer representing the frame number of an event                                                   |

Table 2: Input/output data types of modules in the program executor.

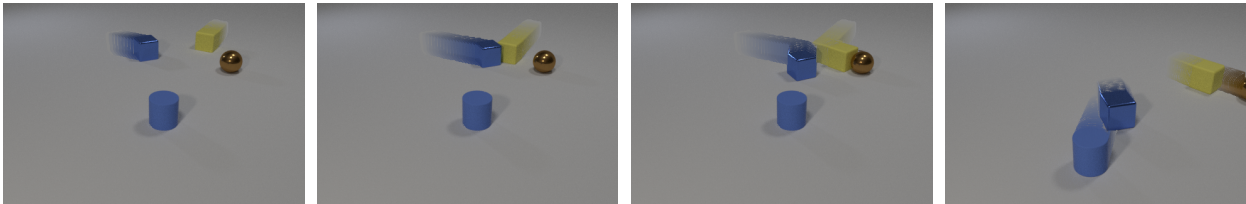

Question: *What is the color of the last object to collide with the blue cube?*

Ground-truth answer: *Blue*

**Video parsing**

|           |          |       |        |        |
|-----------|----------|-------|--------|--------|
| Object ID | 1        | 2     | 3      | 4      |
| Color     | Blue     | Blue  | Brown  | Yellow |
| Material  | Rubber   | Metal | Metal  | Rubber |
| Shape     | Cylinder | Cube  | Sphere | Cube   |

**Motion/event extraction**

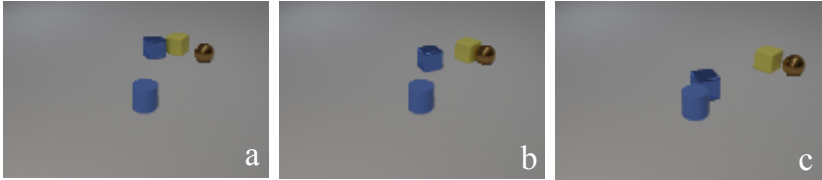

Observed collision events

a: {Frame: 20, Objects: [2,4]}  
b: {Frame: 25, Objects: [3,4]}  
c: {Frame: 50, Objects: [1,2]}

**Question parsing**

Question: *What is the color of the last object to collide with the blue cube?*

Program: `Query_color(Query_partner(Filter_collision(Filter_color(Filter_shape(Objects,Cube), Blue), Last)))`

**Program execution**

|                              |              |           |
|------------------------------|--------------|-----------|
| Module                       | Input        | Output    |
| Events                       | -            | [a,b,c]   |
| Objects                      | -            | [1,2,3,4] |
| Filter_color(_, Blue)        | [1,2,3,4]    | [1,2]     |
| Filter_shape(_, Cube)        | [1,2]        | [2]       |
| Filter_collision(_, _, Last) | ([a,b,c], 2) | [c]       |
| Query_partner(_, _)          | (c, 2)       | 1         |
| Query_color(_)               | 1            | Blue      |

Predicted answer: *Blue*

Figure 2: Running example of DEPICTR on descriptive questions from CLEVRER.

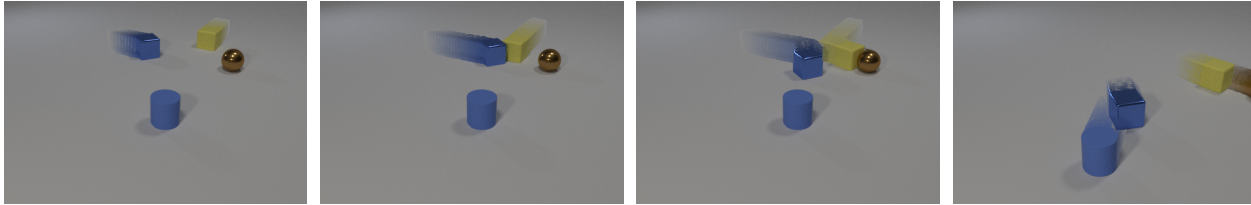

Question: *What is responsible for the sphere's colliding with the yellow cube?*

Option: *The presence of the blue cylinder*

Ground-truth answer: *No*

### Video parsing

| Object ID | 1        | 2     | 3      | 4      |
|-----------|----------|-------|--------|--------|
| Color     | Blue     | Blue  | Brown  | Yellow |
| Material  | Rubber   | Metal | Metal  | Rubber |
| Shape     | Cylinder | Cube  | Sphere | Cube   |

### Motion/event extraction

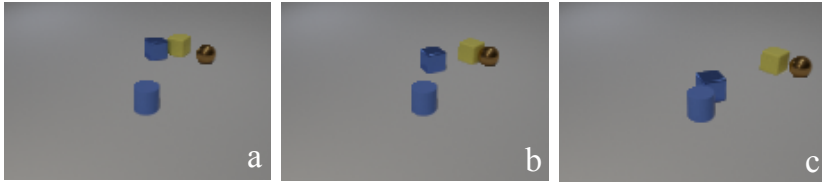

Observed collision events

a: {Frame: 20, Objects: [2,4]}  
b: {Frame: 25, Objects: [3,4]}  
c: {Frame: 50, Objects: [1,2]}

### Question parsing

Question: *What is responsible for the sphere's colliding with the yellow cube?*

Program: `Belong_to(_, Filter_ancestor(Filter_collision(Filter_collision(Events, Filter_shape(Objects, Sphere))), Filter_shape(Filter_color(Objects, Yellow), Cube)))`

Option: *The presence of the blue cylinder*

Program: `Filter_color(Filter_shape(Objects, Cylinder), Blue)`

### Program execution

| Module                    | Input        | Output    |
|---------------------------|--------------|-----------|
| Objects                   | -            | [1,2,3,4] |
| Filter_shape(_, Cylinder) | [1,2,3,4]    | [1]       |
| Filter_color(_, Blue)     | [1]          | [1]       |
| Events                    | -            | [a,b,c]   |
| Objects                   | -            | [1,2,3,4] |
| Filter_shape(_, Sphere)   | [1,2,3,4]    | [3]       |
| Filter_collision(_, _)    | ([a,b,c], 3) | [b]       |
| Objects                   | -            | [1,2,3,4] |
| Filter_color(_, Yellow)   | [1,2,3,4]    | [4]       |
| Filter_shape(_, Cube)     | [4]          | [4]       |
| Filter_collision(_, _)    | ([b], 4)     | [b]       |
| Filter_ancestor(_)        | B            | [a]       |
| Belong_to(_, _)           | (1, [a])     | No        |

Predicted answer: *No*

(Reject the option)

Figure 3: Running example of DEPICTR on explanatory questions from CLEVRER.

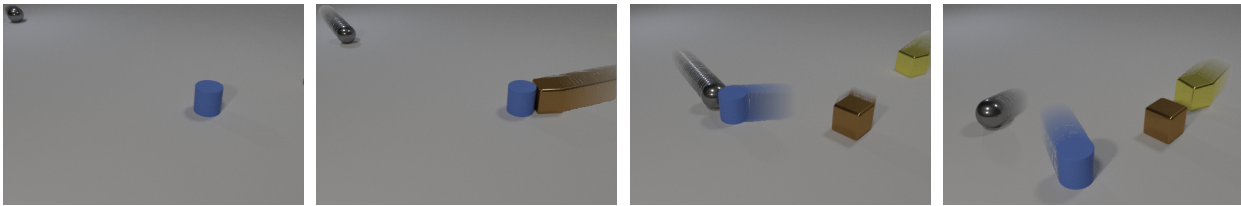

Question: *What will happen next?*  
Option: *The brown cube collides with the yellow object*  
Ground-truth answer: *Yes*

**Video parsing**

| Object ID | 1        | 2      | 3     | 4      |
|-----------|----------|--------|-------|--------|
| Color     | Blue     | Gray   | Brown | Yellow |
| Material  | Rubber   | Metal  | Metal | Metal  |
| Shape     | Cylinder | Sphere | Cube  | Cube   |

**Future motion/event prediction**

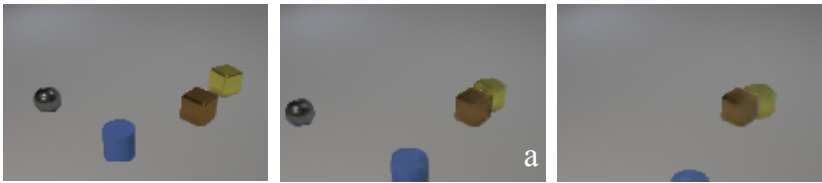

Predicted collision events  
a: {Frame: 145, Objects: [3,4]}

**Question parsing**

Question: *What will happen next?*  
Program: `Belong_to(_, UnseenEvents)`  
Option: *The brown cube collides with the yellow object*  
Program: `Filter_collision(Filter_collision(AllEvents, Filter_shape(Filter_color(Objects, Brown), Cube)), Filter_color(Objects, Yellow))`

**Program execution**

| Module                  | Input                  | Output                         |
|-------------------------|------------------------|--------------------------------|
| AllEvents               | -                      | [all possible collisions]      |
| Objects                 | -                      | [1,2,3,4]                      |
| Filter_color(_, Brown)  | [1,2,3,4]              | [3]                            |
| Filter_shape(_, Cube)   | [3]                    | [3]                            |
| Filter_collision(_, _)  | ([all cols],3)         | [all possible collisions on 3] |
| Objects                 | -                      | [1,2,3,4]                      |
| Filter_color(_, Yellow) | [1,2,3,4]              | [4]                            |
| Filter_collision(_, _)  | ([all cols on 3],4)    | [collision between 3&4]        |
| UnseenEvents            | -                      | [a]                            |
| Belong_to(_, _)         | (col between 3&4, [a]) | Yes                            |

Predicted answer: *Yes*  
(Select the option)

Figure 4: Running example of DEPICTR on predictive questions from CLEVRER.



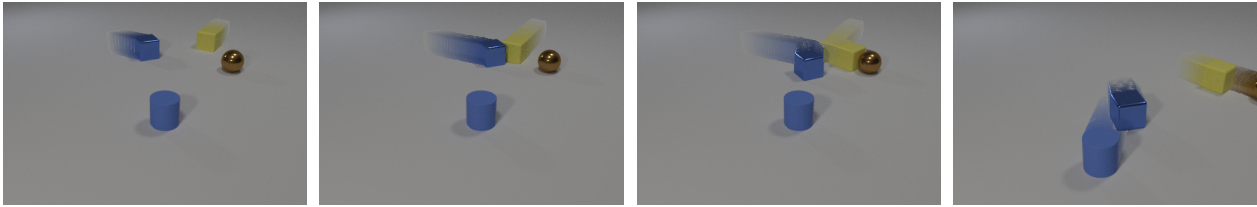

Question: *What will happen without the yellow cube?*

Option: *The blue cube collides with the metal sphere*

Ground-truth answer: Yes

### Video parsing

| Object ID | 1        | 2     | 3      | 4      |
|-----------|----------|-------|--------|--------|
| Color     | Blue     | Blue  | Brown  | Yellow |
| Material  | Rubber   | Metal | Metal  | Rubber |
| Shape     | Cylinder | Cube  | Sphere | Cube   |

### Counterfactual motion/event prediction

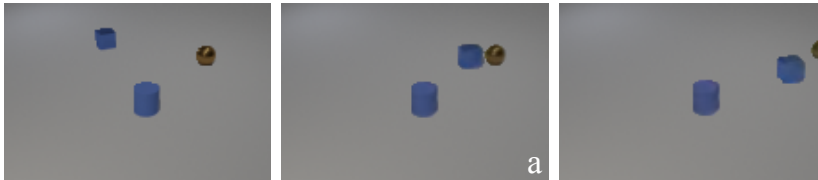

Counterfactual collision events

(Remove yellow rubber cube)

a: {Frame: 25, Objects: [2,3]}

### Question parsing

Question: *What will happen without the yellow cube?*

Program: `Belong_to(_, Get_counterfact(Filter_color(Filter_shape(Objects, Cube), Yellow))`

Option: *The blue cube collides with the metal sphere*

Program: `Filter_collision(Filter_collision(AllEvents, Filter_color(Filter_shape(Objects, Cube), Blue)), Filter_material(Filter_shape(Objects, Sphere), Metal))`

### Program execution

| Module                    | Input                  | Output                         |
|---------------------------|------------------------|--------------------------------|
| AllEvents                 | -                      | [all possible collisions]      |
| Objects                   | -                      | [1,2,3,4]                      |
| Filter_shape(_, Cube)     | [1,2,3,4]              | [2,4]                          |
| Filter_color(_, Blue)     | [2,4]                  | [2]                            |
| Filter_collision(_, _)    | ([all cols],2)         | [all possible collisions on 2] |
| Objects                   | -                      | [1,2,3,4]                      |
| Filter_shape(_, Sphere)   | [1,2,3,4]              | [3]                            |
| Filter_material(_, Metal) | [3]                    | [3]                            |
| Filter_collision(_, _)    | ([all cols on 2],3)    | collision between 2&3          |
| Objects                   | -                      | [1,2,3,4]                      |
| Filter_shape(_, Cube)     | [1,2,3,4]              | [2,4]                          |
| Filter_color(_, Yellow)   | [2,4]                  | [4]                            |
| Get_counterfact(_)        | 4                      | [a]                            |
| Belong_to(_, _)           | (col between 2&3, [a]) | Yes                            |

Predicted answer: Yes

(Select the option)

Figure 5: Running example of DEPICTR on counterfactual questions from CLEVRER.
