# Supplementary material for: CLEVRER: CoLlision Events for Video REpresentation and Reasoning
Source: arXiv:1910.01442 source file (2020-03-08)
Supplement: Supplementary file 5 [file run_example_pred.tex]

\begin{figure}[t]
\includegraphics[width=\linewidth]{fig/supp/running_sim_10000_pred_v3.pdf}
\vspace{-15pt}
\caption{Running example of \model on predictive questions from \data.}
\vspace{-15pt}
\label{fig:exp_pred}
\end{figure}
