# Supplementary material for: CLEVRER: CoLlision Events for Video REpresentation and Reasoning
Source: arXiv:1910.01442 source file (2020-03-08)
Supplement: Supplementary file 7 [file dataset.tex]

\begin{table*}[h]
	\begin{center}
	\begin{tabular}{cc}
	\toprule
	    Sub-type & Answers \\
        \midrule
        \texttt{Count} & \textit{0}, \textit{1}, \textit{2}, \textit{3}, \textit{4}, \textit{5} \\
        \texttt{Exist} & \textit{yes}, \textit{no} \\
        \texttt{Query\_material} & \textit{rubber}, \textit{metal} \\
        \texttt{Query\_shape} & \textit{sphere}, \textit{cube}, \textit{cylinder} \\
        \multirow{2}{*}{\texttt{Query\_color}} & \textit{gray}, \textit{brown}, \textit{green}, \textit{red}, \\
         & \textit{blue}, \textit{purple}, \textit{yellow}, \textit{cyan} \\
    \bottomrule
	\end{tabular}
	\end{center}
	\vspace{-10pt}
	\caption{}
	\vspace{-13pt}
	\label{tab:supp-dataset}
\end{table*}
