# Supplementary material for: CLEVRER: CoLlision Events for Video REpresentation and Reasoning
Source: arXiv:1910.01442 source file (2020-03-08)
Supplement: Supplementary file 9 [file input_modules.tex]

\begin{table}[h]
    \centering
    \small
    \setlength{\tabcolsep}{4pt}
    \begin{tabular}{l l l l}
        \toprule
        Module & Input & Output & Description \\
        \midrule
        \texttt{Objects} & - & \textit{objects} & Returns a list of all object in the video \\
        \texttt{Events} & - & \textit{events} & Returns a list of all events that happened in the video \\
        \texttt{UnseenEvents} & - & \textit{events} & Returns the a list of all future events predicted by the dynamics model \\
        \texttt{AllEvents} & - & \textit{events} & Returns the a list of all possible events on / between any objects \\
        \texttt{Start} & - & \textit{event} & Returns the special ``start" event indicating the start of the video \\
        \texttt{End} & - & \textit{event} & Returns the special ``end" event indicating the end of the video \\
        \bottomrule
    \end{tabular}
    \caption{Input modules of the program executor. The \texttt{UnseenEvents} modules inputs the predictive roll-out results from the dynamics predictor.}
\end{table}
