# Supplementary material for: CLEVRER: CoLlision Events for Video REpresentation and Reasoning
Source: arXiv:1910.01442 source file (2020-03-08)
Supplement: Supplementary file 11 [file output_modules.tex]

\begin{table}[h]
    \centering
    \small
    \setlength{\tabcolsep}{4pt}
    \begin{tabular}{l l l l}
        \toprule
        Module & Input & Output & Description \\
        \midrule
        \texttt{Query\_color} & \textit{object} & \textit{color} & Returns the color of the input object \\
        \texttt{Query\_material} & \textit{object} & \textit{material} & Returns the material of the input object \\
        \texttt{Query\_shape} & \textit{object} & \textit{shape} & Returns the shape of the input object \\
        \texttt{Count} & \textit{objects} & \textit{number} & Returns the number of the input objects \\
        \texttt{Exist} & \textit{objects} & \textit{bool} & Returns ``yes" if the input objects is not empty \\
        \texttt{Not} & \textit{bool} & \textit{bool} & Returns the opposite of the input boolean token \\
        \bottomrule
    \end{tabular}
    \caption{Output modules of the program executor.}
\end{table}
